# Supplementary material for: Complex Absorbing Potential Green's Function Methods for Resonances
Source: arXiv:2507.03496 ancillary file (2025-07-04)
Supplement: Supplementary file 1 [file supporting.pdf]

# Supporting Information for "Complex Absorbing Potential Green's Function Methods for Resonances"

Loris Burth,[1] Fábris Kossoski,[1] and Pierre-François Loos[1,*]

[1] *Laboratoire de Chimie et Physique Quantiques (UMR 5626), Université de Toulouse, CNRS, Toulouse, France*

## I. GEOMETRY FILES

TABLE S1. Cartesian coordinates of the atoms (in Å). X marks the position of the ghost atom at which the additional diffuse basis functions are placed.

$N_2$

| Atom | $x$ | $y$ | $z$ |
|---|---|---|---|
| N | 0.000000 | 0.000000 | −0.548757 |
| N | 0.000000 | 0.000000 | 0.548757 |
| X | 0.000000 | 0.000000 | 0.000000 |

CO

| Atom | $x$ | $y$ | $z$ |
|---|---|---|---|
| C | 0.000000 | 0.000000 | −0.563997 |
| O | 0.000000 | 0.000000 | 0.563997 |
| X | 0.000000 | 0.000000 | 0.000000 |

$C_2H_2$

| Atom | $x$ | $y$ | $z$ |
|---|---|---|---|
| C | 0.000000 | 0.000000 | 0.601489 |
| C | 0.000000 | 0.000000 | −0.601489 |
| H | 0.000000 | 0.000000 | 1.687467 |
| H | 0.000000 | 0.000000 | −1.687467 |
| X | 0.000000 | 0.000000 | 0.000000 |

$C_2H_4$

| Atom | $x$ | $y$ | $z$ |
|---|---|---|---|
| C | 0.669489 | 0.000000 | 0.000000 |
| C | −0.669489 | 0.000000 | 0.000000 |
| H | 1.232054 | 0.928906 | 0.000000 |
| H | −1.232054 | 0.928906 | 0.000000 |
| H | 1.232054 | −0.928906 | 0.000000 |
| H | −1.232054 | −0.928906 | 0.000000 |
| X | 0.000000 | 0.000000 | 0.000000 |

* loos@irsamc.ups-tlse.fr

TABLE S2. Cartesian coordinates of the atoms (in Å). X marks the position of the ghost atom at which the additional diffuse basis functions are placed.

$CH_2O$

| Atom | $x$ | $y$ | $z$ |
|---|---|---|---|
| C | 0.000000 | 0.000000 | −0.007698 |
| O | 0.000000 | 0.000000 | 1.197292 |
| H | 0.943214 | 0.000000 | −0.594797 |
| H | −0.943214 | 0.000000 | −0.594797 |
| X | 0.000000 | 0.000000 | 0.000000 |

$CO_2$

| Atom | $x$ | $y$ | $z$ |
|---|---|---|---|
| O | 0.000000 | 0.000000 | −1.163026 |
| C | 0.000000 | 0.000000 | 0.000000 |
| O | 0.000000 | 0.000000 | 1.163026 |
| X | 0.000000 | 0.000000 | 0.000000 |

## II. ADDITIONAL DIFFUSE BASIS FUNCTIONS

Additional basis functions that we added to the aug-cc-pVTZ basis sets. For the derivation, we refer to the computational details section in the main text.

TABLE S3. Additional diffuse basis functions for $N_2$, CO, $C_2H_2$ and $C_2H_4$.

$N_2$

| Type | Exponent |
|---|---|
| S | 0.0288000 |
| S | 0.0144000 |
| S | 0.0072000 |
| P | 0.0245500 |
| P | 0.0122750 |
| P | 0.0061375 |
| D | 0.0755000 |
| D | 0.0377500 |
| D | 0.0188750 |

CO

| Type | Exponent |
|---|---|
| S | 0.029445000 |
| S | 0.014722500 |
| S | 0.007361250 |
| P | 0.023857500 |
| P | 0.011928750 |
| P | 0.005964375 |
| D | 0.078500000 |
| D | 0.039250000 |
| D | 0.019625000 |

$C_2H_2$

| Type | Exponent |
|---|---|
| S | 0.02201000 |
| S | 0.01100500 |
| S | 0.00550250 |
| P | 0.01784500 |
| P | 0.00892250 |
| P | 0.00446125 |
| D | 0.05000000 |
| D | 0.02500000 |
| D | 0.01250000 |

$C_2H_4$

| Type | Exponent |
|---|---|
| S | 0.02201000 |
| S | 0.01100500 |
| S | 0.00550250 |
| P | 0.01784500 |
| P | 0.00892250 |
| P | 0.00446125 |
| D | 0.05000000 |
| D | 0.02500000 |
| D | 0.01250000 |

TABLE S4. Additional diffuse basis functions for $CH_2O$ and $CO_2$.

| $CH_2O$ | | $CO_2$ | |
|---|---|---|---|
| Type | Exponent | Type | Exponent |
| S | 0.029445000 | S | 0.029445000 |
| S | 0.014722500 | S | 0.014722500 |
| S | 0.007361250 | S | 0.007361250 |
| P | 0.023857500 | P | 0.023857500 |
| P | 0.011928750 | P | 0.011928750 |
| P | 0.005964375 | P | 0.005964375 |
| D | 0.078500000 | D | 0.078500000 |
| D | 0.039250000 | D | 0.039250000 |
| D | 0.019625000 | D | 0.019625000 |

## III. DYSON ORBITALS

All the visualizations in this section are performed with *Pegamoid 2.12.3*. They are shown with the molecular plane oriented perpendicular to the plane of the page (i.e., the viewing plane). The pictures visualize molecular orbitals in a cube of edge length 30 $a_0$ with a isovalue 0.004.

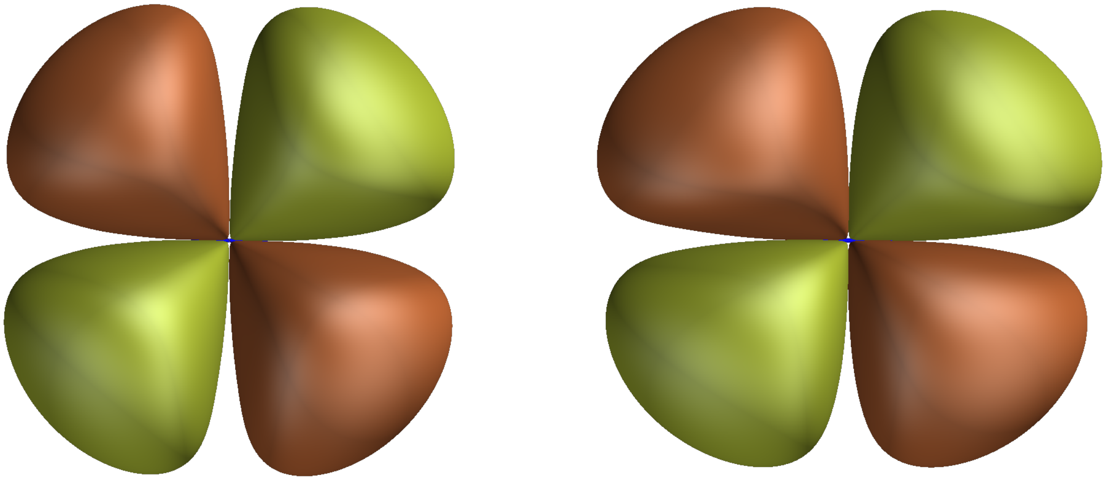

FIG. S1. Real part of the Dyson orbital of the $^2\Pi_g$ resonance state of $N_2{}^-$ derived by CAP augmented qs$GW$ at $\eta = 0.0016$ a.u. (left panel) $\eta = 0.0078$ a.u. (right panel).

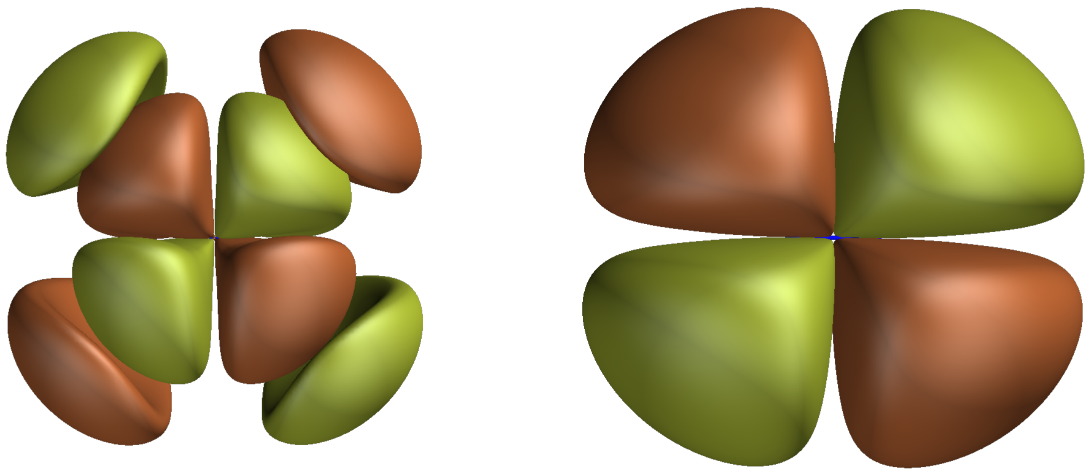

FIG. S2. Real part of the Dyson orbital of the $^2\Pi_g$ resonance state of $N_2{}^-$ derived by CAP augmented HF, corresponding to $G_0W_0$ and ev$GW$, at $\eta = 0.0017$ a.u. (left panel) $\eta = 0.0115$ a.u. (right panel).

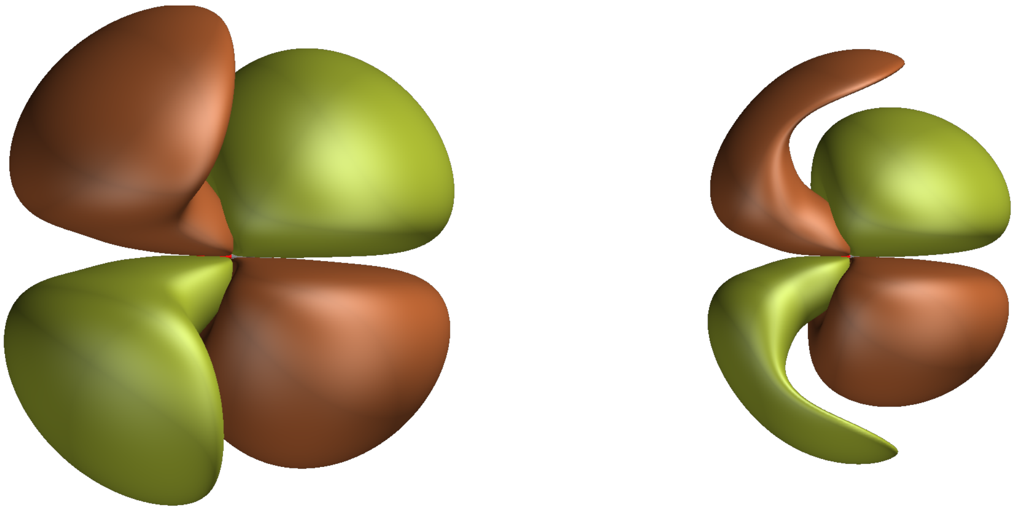

FIG. S3. Real part of the Dyson orbital of the $^2\Pi$ resonance state of $CO^-$ derived by CAP augmented HF, corresponding to $G_0W_0$ at 0.008 70 a.u. (left panel) and derived by qs$GW$, at $\eta = 0.002\,95$ a.u. (right panel).

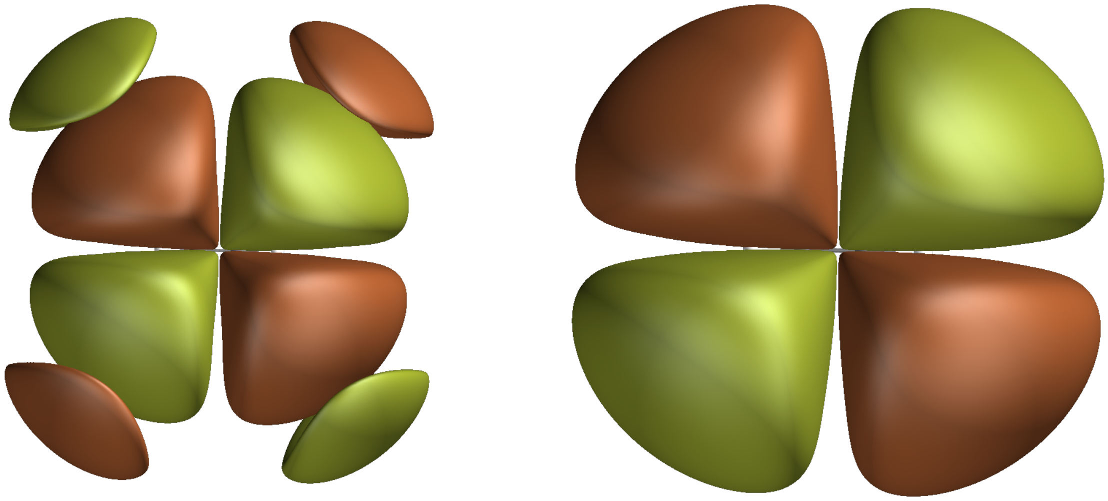

FIG. S4. Real part of the Dyson orbital of the $^2\Pi_g$ resonance state of $C_2H_2{}^-$ derived by CAP augmented HF, corresponding to $G_0W_0$ at 0.0037 a.u. (left panel) and derived by qs$GW$, at $\eta = 0.003\,75$ a.u. (right panel).

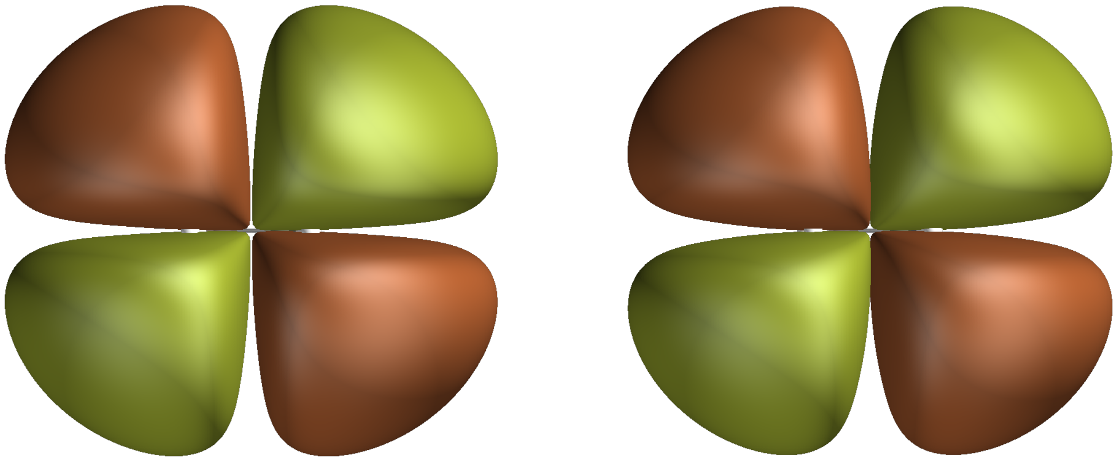

FIG. S5. Real part of the Dyson orbital of the $^2B_{2g}$ resonance state of $C_2H_4{}^-$ derived by CAP augmented HF, corresponding to $G_0W_0$ at 0.012 15 a.u. (left panel) and derived by qs$GW$, at $\eta = 0.004\,75$ a.u. (right panel).

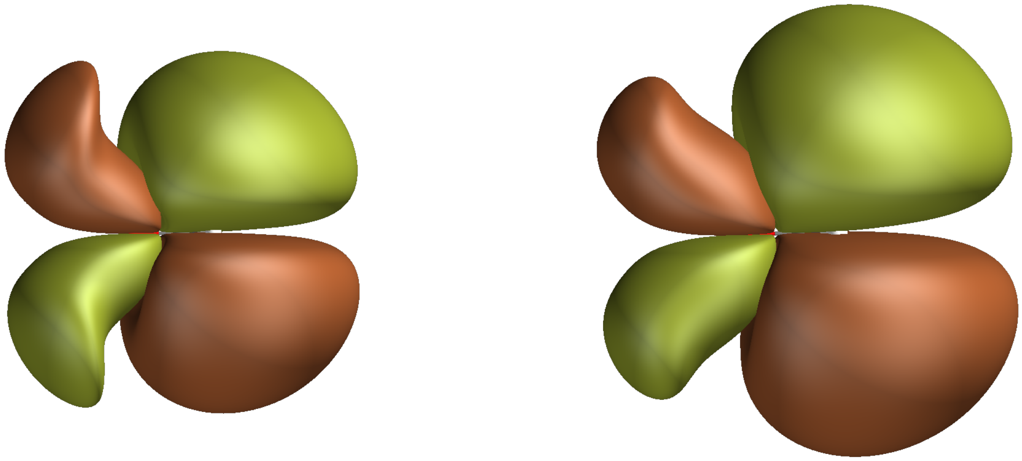

FIG. S6. Real part of the Dyson orbital of the $^2B_1$ resonance state of $CH_2O^-$ derived by CAP augmented HF, corresponding to $G_0W_0$ at $0.009\,15$ a.u. (left panel) and derived by qs$GW$, at $\eta = 0.0045$ a.u. (right panel).

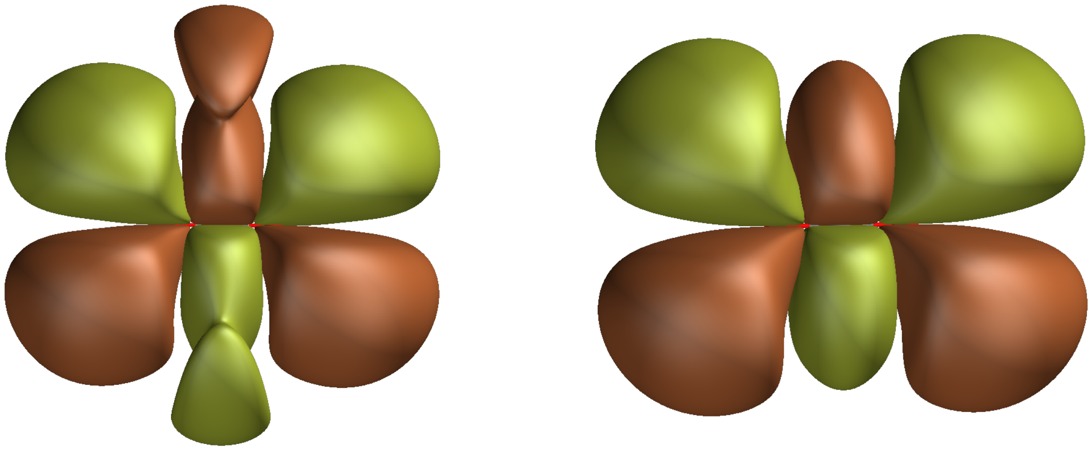

FIG. S7. Real part of the Dyson orbital of the $^2\Pi_u$ resonance state of ${CO_2}^-$ derived by CAP augmented HF, corresponding to $G_0W_0$ at $0.0125$ a.u. (left panel) and derived by qs$GW$, at $\eta = 0.001\,235$ a.u. (right panel).

## IV. ENERGY VELOCITIES

Energy velocities with marked minima. For computational details, see the main text. Note that not all markers are represented for the sake of visibility.

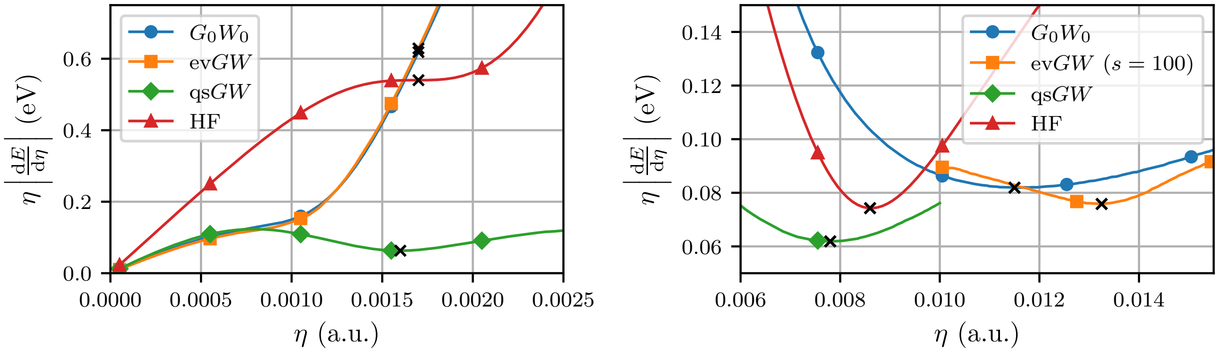


FIG. S8. Energy velocities for $N_2^-$; first minimum (left) and second minimum (right).

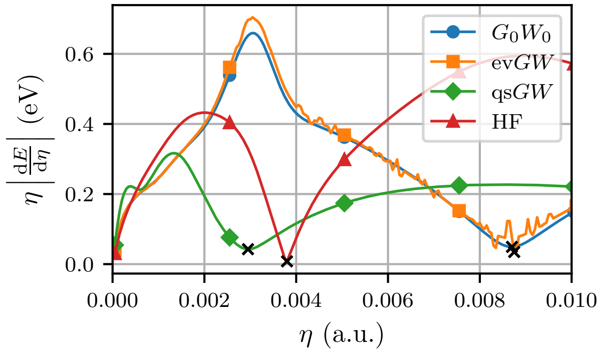


FIG. S9. Energy velocities for $CO^-$.

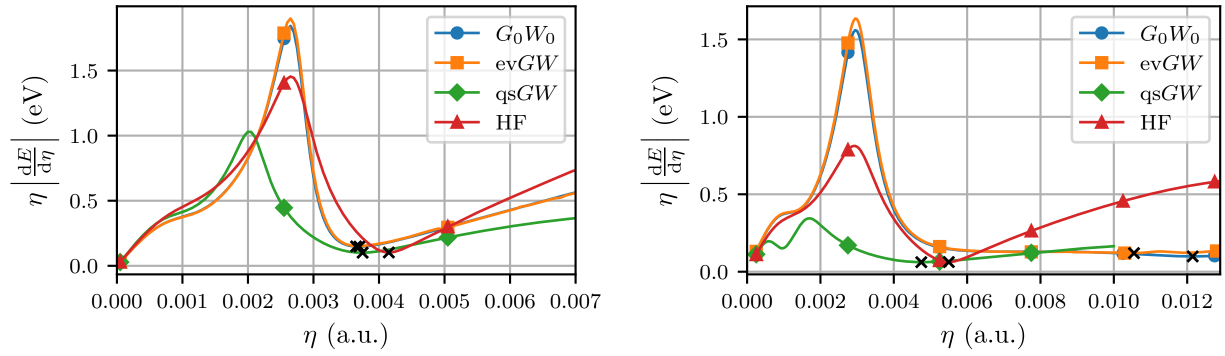


FIG. S10. Energy velocities for $C_2H_2{}^-$ (left) and $C_2H_4{}^-$ (right).

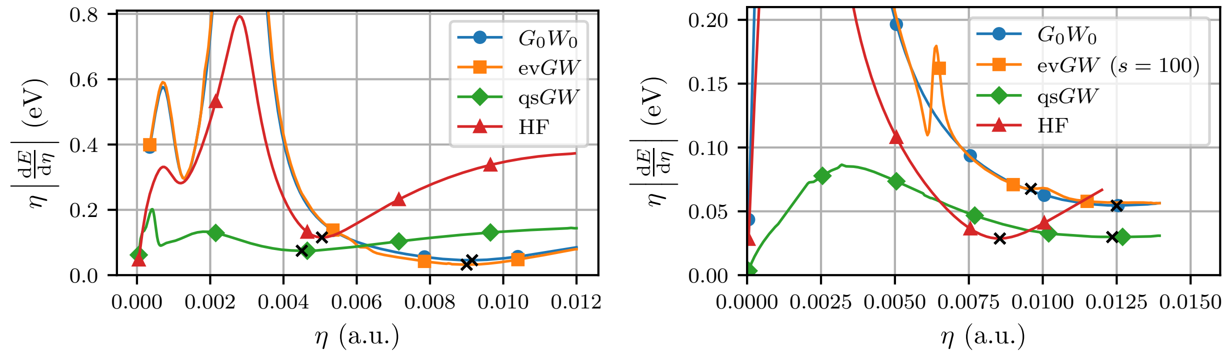


FIG. S11. Energy velocities for $CH_2O^-$ (left) and $CO_2{}^-$ (right).

## V. SPECTRAL FUNCTIONS

Spectral functions of each system for the CAP augmented $G_0W_0$ and qs$GW$ method compared with the broadened spectrum derived by qs$GW$ calculation without CAP. The CAP calculations are performed at the in the main text reported corresponding optimal $\eta$ values.

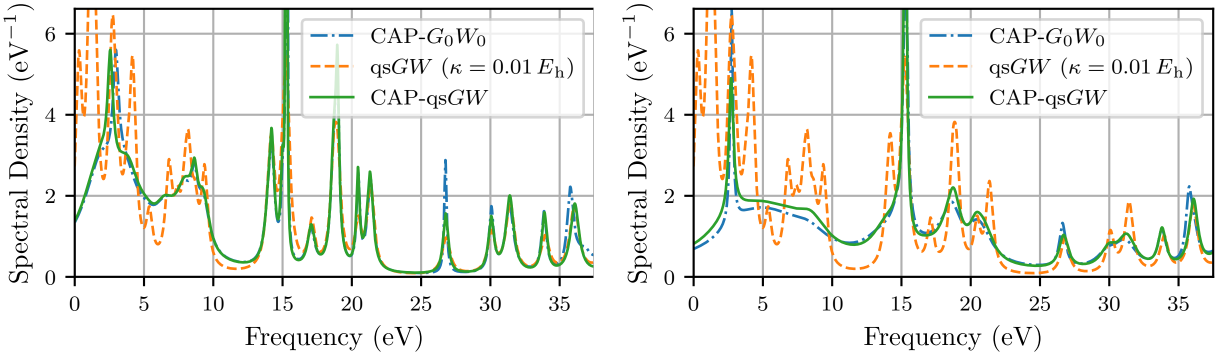


FIG. S12. Spectral functions for $N_2$ at the first minimum (left) and the second minimum (right).

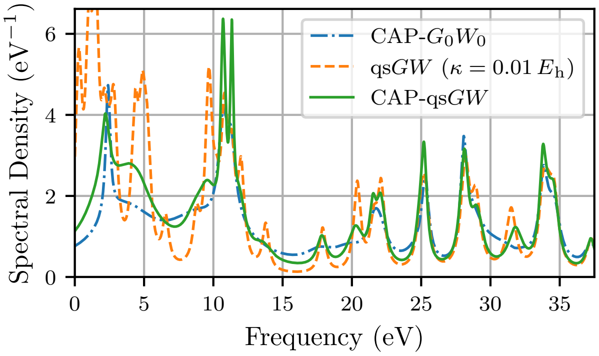


FIG. S13. Spectral functions for CO.

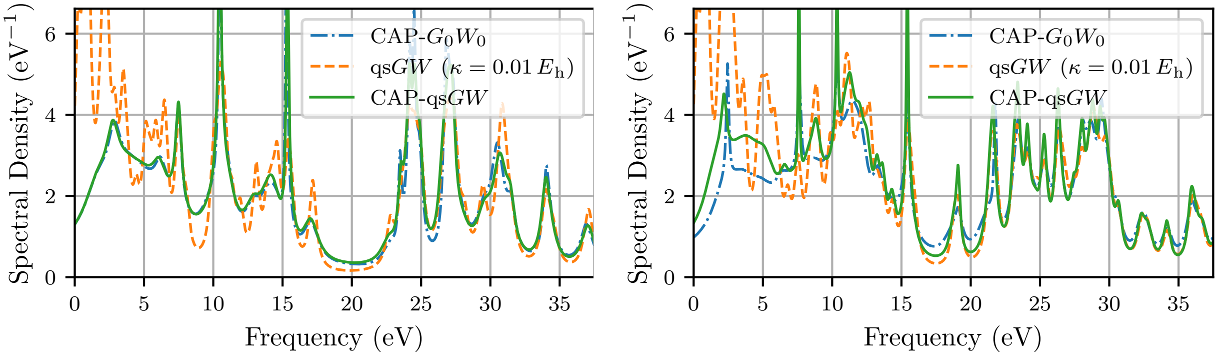


FIG. S14. Spectral functions for $C_2H_2$ (left) and $C_2H_4$ (right).

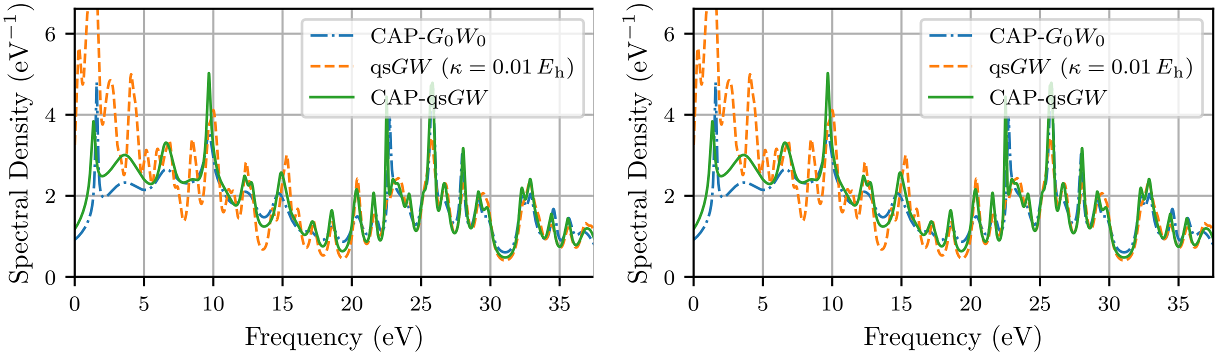


FIG. S15. Spectral functions for $CH_2O$ (left) and $CO_2$ (right).
